# Supplementary material for: Scaling Properties of Continuous Diffusion Spoken Language Models
Source: arXiv:2604.24416 source file (2026-04-27)
Supplement: Supplementary file 1 [file 99_appendix.tex]

\section{Continuous Diffusion SLMs Ablations}
\label{sec:ablations}
To understand the sensitivity of our model to key design choices, we conduct a systematic ablation study across four axes: training duration, temporal patch size, noise schedule, and diffusion timestep discretization. Each ablation isolates a single variable while holding others fixed at default values. We evaluate all configurations using both reference-based metrics (FAD) and reference-free perceptual quality estimators (DNSMOS P.808, NISQA MOS), supplemented by human-aligned aesthetic scores (Content Enjoyment, Content Understanding, Production Quality) and phonetic fidelity (Phoneme \gls{jsd}). To assess the interaction with inference-time guidance, we report results at two \gls{cfg} scales: 2.2, 4.0. For all ablations we train our model with $d_{\text{emb}}$=1024 with 8 layers. We tune the base model hyper-parameters using a sweep over learning rate, weight decay and Adam $\beta_1, \beta_2$ and $\epsilon$.
\subsection{Training Duration}
\label{sec:ablation_duration}
\textbf{NB(jrp): do we need this section given scaling laws?}
We first examine how generation quality evolves with training compute, measured in cumulative hours of audio processed. Training spans from 0.25M to 1.5M hours in increments of 0.25M hours. Figure~\ref{fig:ablation_duration} summarizes these results.
\begin{figure}[htbp]
  \centering
  \includegraphics[width=\linewidth]{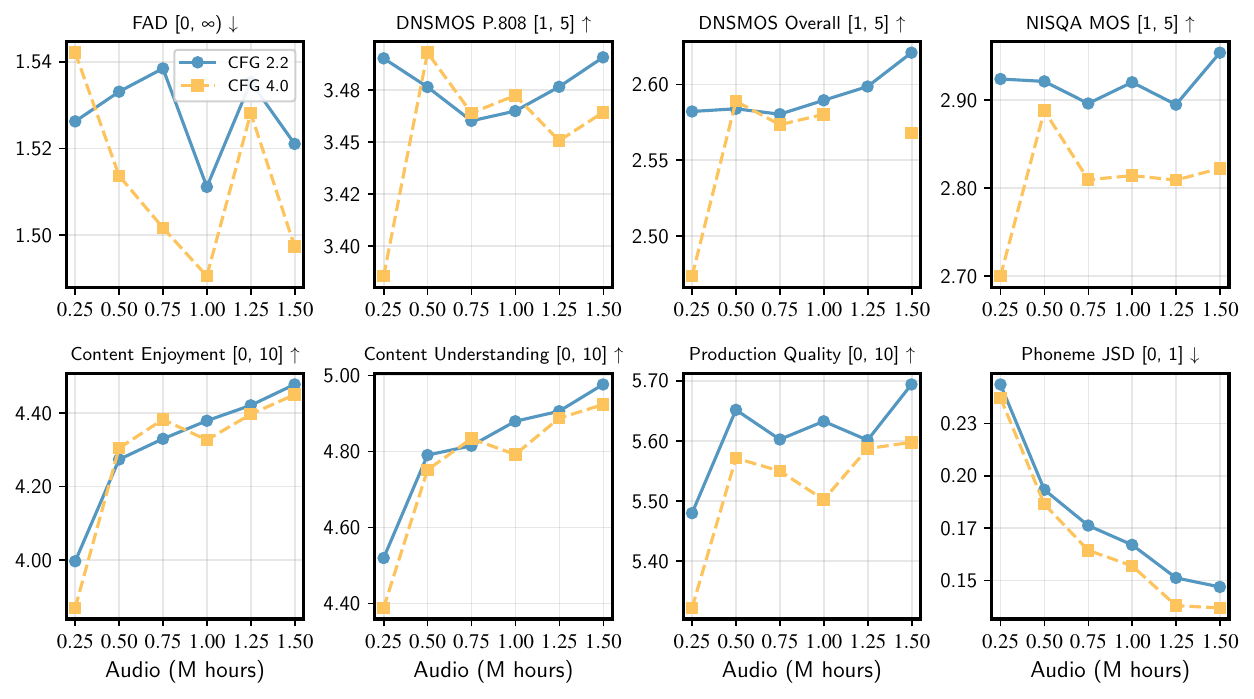}
  \caption{Effect of training duration on audio quality. All metrics improve monotonically with increased audio data.}
  \label{fig:ablation_duration}
\end{figure}
Perceptual quality metrics exhibit clear monotonic improvement with increased training. Content Enjoyment rises from 4.0 to 4.5 and Production Quality from 5.4 to 5.7 as training progresses from 0.25M to 1.5M hours. Phoneme JSD decreases correspondingly, indicating improved phonetic accuracy. In contrast, FAD and DNSMOS show more modest gains and plateau beyond 1.0M hours, suggesting that reference-based metrics saturate earlier than subjective quality measures. \textbf{TODO: describe VGGish FAD model.} Throughout training, CFG~2.2 maintains a consistent advantage over CFG~4.0 across most metrics, with particularly pronounced differences in NISQA MOS.

\subsection{Temporal Patch Size}
\label{sec:ablation_patch_size}
Analogous to spatial patching in vision transformers, we investigate temporal patching of Mel filterbanks, where a patch size of $k$ folds the temporal dimension by a factor of $k$ while proportionally expanding the channel dimension. This reduces sequence length and computational cost but potentially sacrifices fine-grained temporal resolution. Figure~\ref{fig:ablation_patch_size} presents results across patch sizes 1--6.
\begin{figure}[htbp]
  \centering
  \includegraphics[width=\linewidth]{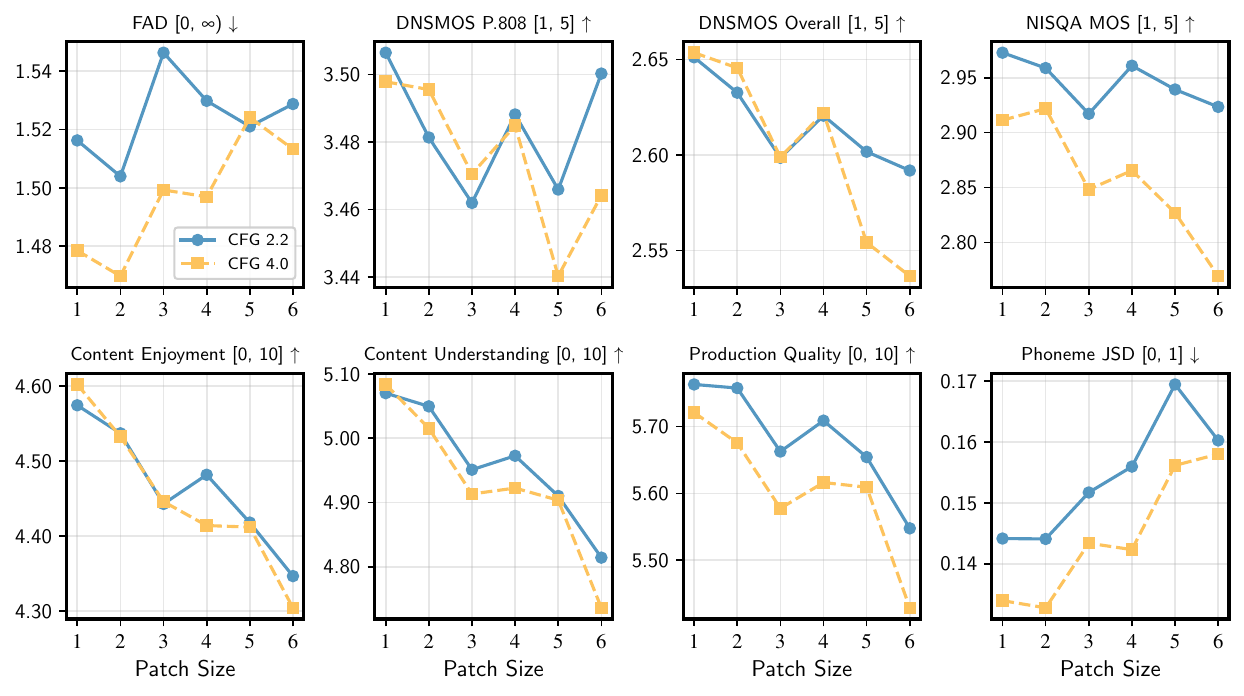}
  \caption{Effect of temporal patch size on audio quality. Smaller patches preserve fine-grained temporal structure, yielding consistently better perceptual quality.}
  \label{fig:ablation_patch_size}
\end{figure}

The results reveal a consistent pattern: smaller patch sizes yield superior quality across nearly all metrics. A patch size of 1 (no folding) achieves the highest Content Enjoyment (4.57), Content Understanding (5.08), and Production Quality (5.77). Quality degrades progressively as patch size increases, with patch sizes of 5--6 showing notably worse performance. 

These findings suggest that temporal resolution is critical for high-fidelity audio generation. While larger patch sizes offer computational savings, the quality degradation may be unacceptable for applications requiring natural prosody and fine temporal detail. We recommend patch size 1 for quality-critical applications and patch size 2 as a reasonable efficiency compromise.

\subsection{Noise Schedule}
\label{sec:ablation_noise_schedule}
The noise schedule determines how the signal-to-noise ratio (SNR) changes over diffusion timesteps, and thus which noise levels dominate the learning problem and the denoising trajectory at sampling time. Because classifier-free guidance (\gls{cfg}) is applied only during inference, schedule choice should be interpreted jointly with the intended guidance regime: increasing \gls{cfg} is not better in general, but an application-driven dial that trades off stronger adherence to the conditioning signal against diversity and naturalness. For this reason, the results at CFG~2.2 and CFG~4.0 are not competing recommendations for a single setting; they are measurements of the same schedule ablation under two different sampling regimes.
We evaluate three schedules (linear, cosine, exponential), each with and without zero terminal SNR (enforcing complete signal destruction at $t=T$)~\cite{DBLP:conf/wacv/LinLLY24}. Each cell in Figures~\ref{fig:ablation_noise_cfg22} and~\ref{fig:ablation_noise_cfg40} corresponds to a separately trained model using that schedule; the only difference between the figures is the fixed \gls{cfg} used during evaluation.
\begin{figure}[htbp]
  \centering
  \includegraphics[width=\linewidth]{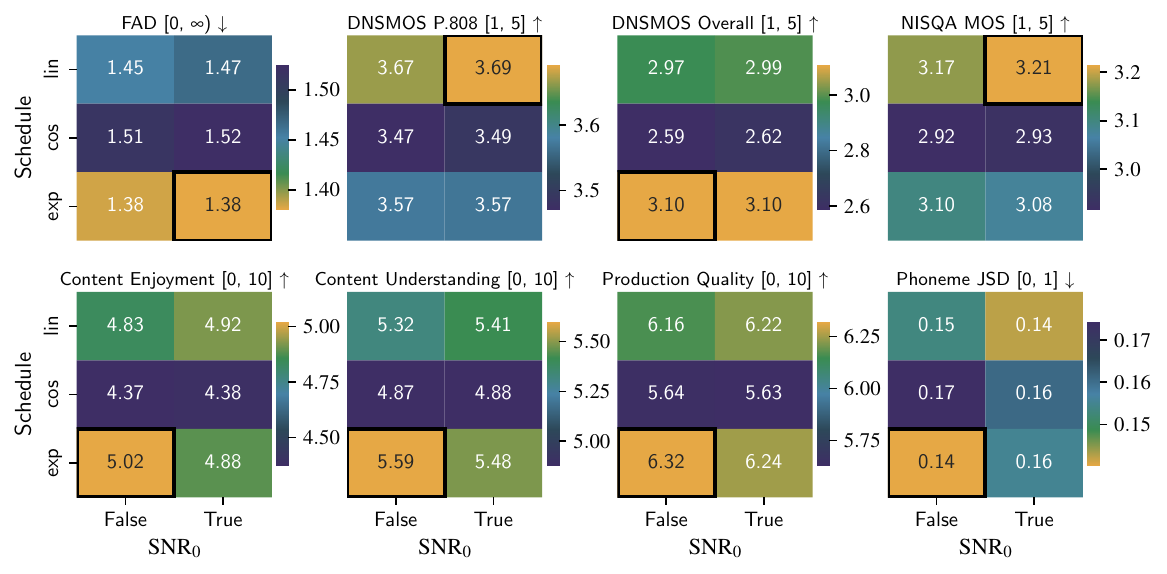}
  \caption{Noise schedule ablation at \gls{cfg}~2.2 (moderate guidance). Each cell is a separately trained model and shows the metric value for a schedule type and terminal SNR setting. Black borders indicate optimal configurations. In this regime the exponential schedule training dominates.}
  \label{fig:ablation_noise_cfg22}
\end{figure}
\begin{figure}[htbp]
  \centering
  \includegraphics[width=\linewidth]{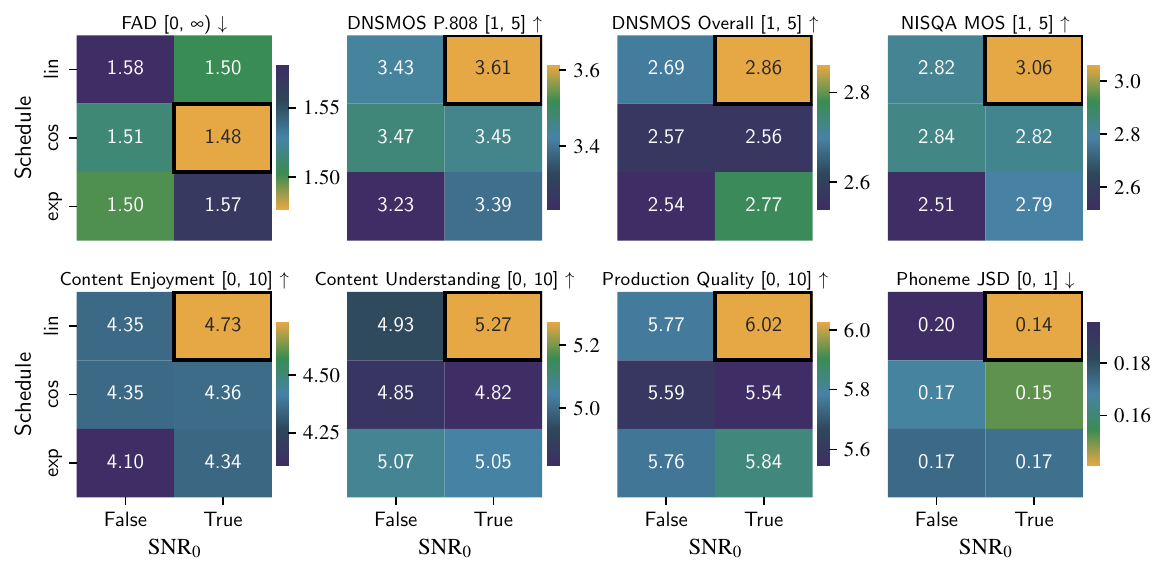}
  \caption{Noise schedule ablation evaluated at \gls{cfg}~4.0 (stronger guidance). Under stronger guidance, linear schedules (especially with zero terminal SNR) dominate most perceptual and aesthetic metrics, while exponential schedules no longer lead.}
  \label{fig:ablation_noise_cfg40}
\end{figure}
Two conclusions are stable across guidance regimes. First, the cosine schedule is consistently uncompetitive, trailing linear and exponential alternatives on perceptual and aesthetic predictors. Second, zero terminal SNR is most helpful in combination with the linear schedule, suggesting that explicitly training for complete signal destruction improves robustness at the high-noise end of the trajectory.

Beyond these, the preferred schedule depends on how the model will be sampled. At moderate guidance (CFG~2.2), exponential schedules achieve the best distributional alignment (lowest FAD) and strong aesthetic scores, while linear with zero terminal SNR yields the best MOS-predicted perceptual quality (DNSMOS P.808 and NISQA). At stronger guidance (CFG~4.0), the ordering shifts: linear with zero terminal SNR becomes the most reliable choice across perceptual, aesthetic, and phonetic metrics, and exponential schedules degrade.

One interpretation is that stronger guidance amplifies sensitivity to modeling error at high noise levels; in that regime, a schedule that better supports early, high-noise denoising (and explicitly reaches SNR$(T)=0$) is advantageous. Practically, we therefore treat the noise schedule as part of the inference configuration: linear with zero terminal SNR is a robust default when sampling with higher \gls{cfg}, while exponential schedules remain competitive at lower \gls{cfg}. 

\subsection{Diffusion Timesteps}
\label{sec:ablation_timesteps}
The number of diffusion timesteps $T$ determines the granularity of the noise level discretization during training. Finer discretization (larger $T$) provides more precise noise level targets but increases the complexity of the learning problem. We train multiple models with $T \in \{100, 500, 1000, 2000, 4000\}$, and evaluate them using $100$ steps at generation time, with results shown in Figure~\ref{fig:ablation_timesteps}.
\begin{figure}[htbp]
  \centering
  \includegraphics[width=\linewidth]{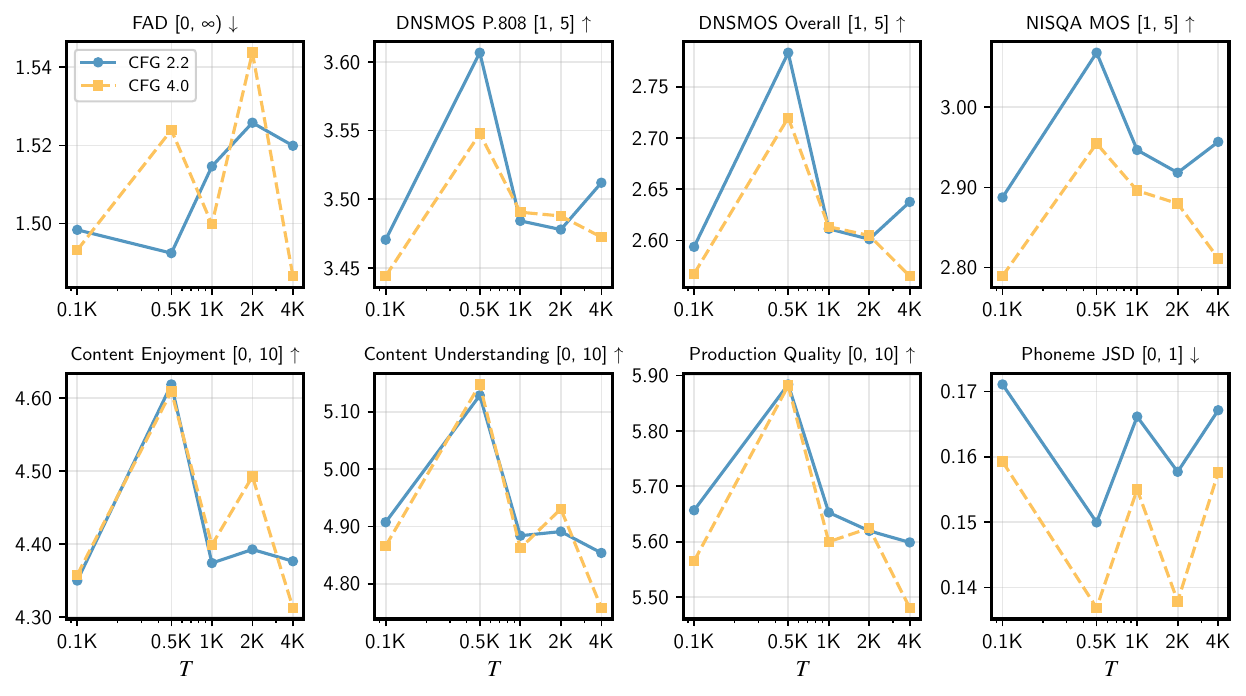}
  \caption{Effect of diffusion timesteps $T$ on audio quality. An optimum emerges at $T=500$, with both coarser and finer discretizations yielding degraded performance.}
  \label{fig:ablation_timesteps}
\end{figure}

\textbf{TODO: need more seeds to make a conclusive statement.}
The results reveal a non-monotonic relationship between $T$ and generation quality. Rather than observing the expected trade-off between discretization granularity and training stability, we find an optimum at $T=500$. At this setting, DNSMOS P.808 reaches 3.61, a substantial improvement over both $T=100$ (3.47) and $T=1000$ (3.48). Similar patterns appear across Content Enjoyment, Content Understanding, and Production Quality, all peaking sharply at $T=500$.

This sweet spot suggests that $T=500$ strikes an effective balance: sufficient discretization to capture the continuous diffusion process while avoiding the optimization difficulties that may arise with finer discretizations. The degradation at larger $T$ values is particularly interesting, as conventional wisdom might suggest that finer discretization should improve or at least maintain quality. We speculate that very large $T$ may introduce training difficulties or cause the model to overfit to specific noise levels. For \gls{cfg}~4.0, the pattern persists but with shifted optima and generally lower absolute performance, reinforcing the advantage of moderate guidance scales. We recommend $T=500$ as the default setting.
